# Supplementary material for: Predicting Stochastic Human Forward Reachable Sets Based on Learned Human Behavior
Source: arXiv:1903.07738 source file (2019-03-18)
Supplement: Supplementary file 1 [file appendix.tex]

\section*{Appendix}

\begin{thm}
\label{thm:reachset_property}
Based on this reachable set generation scheme, 
If for any $j \in \set{1, \dots, \numfreachset-1}$, $\epsilon_j \leq 
\epsilon_{j+1}$ and $\forall j \in \set{1, \dots, \numfreachset}, \epsilon_j
\geq 0$, for any $j \in
\set{1, \dots, \numfreachset-1}$, $\freachset_{j} \subseteq \freachset_{j+1}$ 
% Note that here we define $\freachset_{j} = \freachset_{j}(t_T)$. 
\end{thm}
\noindent \begin{proof}
  First, observe that if $\forall j \in \set{1, \dots, \numfreachset-1}$, $\epsilon_j \leq
  \epsilon_{j+1}$, then at each time step $i \in
  \set{0, \dots, T-1}$, $\underline{u}_{j+1}^{(i)} \leq \underline{u}_{j}^{(i)}$
  and $\bar{u}_{j}^{(i)} \leq \bar{u}_{j+1}^{(i)}$. Equivalently, the control
  input sets at each time step satisfy $U_j^{(i)} = [\underline{u}_{j}^{(i)}
  \bar{u}_{j}^{(i)}] \subseteq [\underline{u}_{j+1}^{(i)} \bar{u}_{j+1}^{(i)}]
  = U_{j+1}^{(i)}$.

  Then consider any two initial sets and input bounds for reachable sets
  $\freachset_a$, $\freachset_b$ that satisfy $\mathcal{L}_a \subseteq
  \mathcal{L}_b$ and $U_a \subseteq U_b$ between time $[t_s,t_e]$ where $t_s$
  and $t_e$ indicate the start and end time respectively. If $x_a \in
  \mathcal{F}_a$, then by definition $\exists u(t) \in U_a$, s.t. $t \in [t_s,
  t_e]$, $x(\cdot) \text{ satisfies } \dot{x} = f(x,u), x(t_s) \in \mathcal{L}_a,
  x(t) = x_a$. Since $U_a \subseteq U_b$ and $\mathcal{L}_a \subseteq
  \mathcal{L}_b$, this means that $u(t) \in U_b$, $t \in [t_s,t_e]$, and $x(t_s) \in
  \mathcal{L}_b$. Hence by definition, $x_a \in \freachset_b$. This proves that
  $\freachset_a \subseteq \freachset_b$.
  % $\mathcal{F}_a = \set{x:  \exists u(t) \in U_a \text{ s.t. }, t
  % \in [t_{s}, t_{e}], x(\cdot) \text{ satisfies } \dot{x} = f(x,u), x(t_s) \in
  % \mathcal{L}_a, x(t) = x}$ and 
  % $\mathcal{F}_b = \set{x:  \exists u(t) \in U_b \text{ s.t. }, t
  % \in [t_{s}, t_{e}], x(\cdot) \text{ satisfies } \dot{x} = f(x,u), x(t_s) \in
  % \mathcal{L}_b, x(t) = x}$, we have $\mathcal{F}_a \subseteq \mathcal{F}_b$.

  We let $\mathcal{F}_j(t_i)$ denote the reachable set $j$ grown so far from
  time $t_0$ to time $t_i$. Using the above result, we have $\mathcal{F}_j(t_1) \subseteq
  \mathcal{F}_{j+1}(t_1)$ because $\mathcal{F}_j(t_0) = \mathcal{F}_{j+1}(t_0)
  = \mathcal{L}$ and $U_{j}^{(0)} \subseteq U_{j+1}^{(0)}$. Then applying this recursively, we have $\mathcal{F}_j(t_i)
  \subseteq \mathcal{F}_{j+1}(t_i)$ for any $i \in \set{2, \dots, T}$. Hence
  $\mathcal{F}_j \subseteq \mathcal{F}_{j+1}$, $\forall j \in \set{1, \dots,
  \numfreachset-1}$.
\end{proof}

We now present how we compute $p_j, j \in \set{1, \dots, \numfreachset}$.
Suppose we have a dataset of $K$ trajectories, denoted as
$\set{\zeta_k}_{k=1}^{K}$. Each trajectory consists of the state
of $\veh_{\mathcal{H}}$ for $L_k$ consecutive time
steps where $L_k \geq T + 1$, i.e., $\zeta_k = \set{x_{\mathcal{H},k}^{(l)}
}_{l=0}^{L_k-1}$. Then for trajectory $k$, we have 
data available to predict $L_k-T$ SHFRS's as we can
predict the next $T$ states starting at time step $l=0, \dots, L_k-T-1$. We let
the segment of trajectory $k$ from time step $l$ to $l+T$ be
denoted as $\zeta_{k,l}$. We let $\freachset_{j,k,l}$ be the $\freachset_j$
generated by starting at the $l$th time step in trajectory $k$. Then we compute
$p_j$ by letting
\vspace{-0.5em}
\begin{equation*}
  p_j = \frac{1}{\sum_{k=1}^{K} (L_k-T)} \sum_{k=1}^{K} \sum_{l=0}^{L_k-T-1}
  \mathds{1}\{\zeta_{k,l} \in \freachset_{j,k,l}
    \}
  \vspace{-.5em}
\end{equation*}
Note here we use a slight abuse of
notation and define $\zeta_{k,l} \in \freachset_{j,k,l}$ if and only if 
$x_{\mathcal{H},k}^{(l)}, \dots, x_{\mathcal{H},k}^{(l+T)} \in
\freachset_{j,k,l}$.

% Intuitively, $p_j$ represents the percentage of trajectory segments that falls
% entirely within $\freachset_j$.
% 
\begin{corr}
  Using our algorithm, $p_{\freachset_{j+1}} \geq p_{\freachset_j}, \forall j \in
  \set{1,\dots,\numfreachset-1}.$
\end{corr}
\begin{proof}
  According to Theorem \ref{thm:reachset_property}, we have that for any $j \in
  \set{1, \dots, \numfreachset-1}$, $\freachset_{j} \subseteq \freachset_{j+1}$.
  This suggests that if $\zeta_{k,l} \in \freachset_{j,k,l}$, then $\zeta_{k,l}
  \in \freachset_{j+1,k,l}$.
  Hence, $\forall k \in \set{1, \dots, K}, \forall l \in \set{0,\dots,L_k-T-1},
  \mathds{1}\{\zeta_{k,l} \in \freachset_{j,k,l}\}
  \leq \mathds{1}\{\zeta_{k,l} \in \freachset_{j+1,k,l}\}$. Hence, $p_{\freachset_j}
  \leq p_{\freachset_{j+1}}, \forall j \in \set{1,\dots,\numfreachset-1}.$
\end{proof}

\begin{corr}
  If we set $\epsilon_{\numfreachset}$ such that 
  $\underline{u}_{\numfreachset}^{(i)} = u_{min},
  \bar{u}_{\numfreachset}^{(i)} = u_{max}, \forall i \in \set{0,\dots,T-1}$, 
  then $p_{\freachset_{\numfreachset}} = 1$.
\end{corr}
\begin{proof}
  Since human inputs are constrained within $[u_{min}, u_{max}]$, any 
  human trajectory must fall inside the forward reachable set where the bounds
  on the inputs are always $[u_{min}, u_{max}]$. Hence if 
  $\underline{u}_{\numfreachset}^{(i)} = u_{min},
  \bar{u}_{\numfreachset}^{(i)} = u_{max}$, then $\zeta_{k,l} \in
  \freachset_{\numfreachset,k,l}, \forall k \in
  \set{1, \dots, K}, \forall l \in \set{0,\dots,L_k-T-1}$. Thus, $p_{\freachset_{\numfreachset}} = 1$.
\end{proof}

Having $\sum_{j=1}^{\numfreachset} p_{\sfreachset_{j}} =
p_{\freachset_{\numfreachset}} = 1$ allows us to capture all possible future
trajectories and provides us with the ability to use 
$\freachset_{\numfreachset}$ as the most conservative safety standard.
